# Supplementary material for: Gaussian Approximation of Convex Sets by Intersections of Halfspaces
Source: arXiv:2311.08575 source file (2023-11-14)
Supplement: Supplementary file 1 [file convex-influences-appendix.tex]

%!TEX root = ../polytope-approximation.tex

\section{Proofs of \Cref{prop:influence-width-ub,prop:size-to-width}}
\label{appendix:polytope-influence-bounds}

We start by proving~\Cref{prop:influence-width-ub}:

\begin{proofof}{\Cref{prop:influence-width-ub}}
	Suppose $K$ is the intersection of halfspaces $\{H_i\}_{i\in\N}$ where 
	\[H_i := \cbra{x\in\R^n : \abra{x, v^{(i)}} \leq \theta_i}\]
	for unit vectors $v^{(i)} \in \S^{n-1}$ and $\theta_i \in \R$.
	Define the sets 
	\[\mathrm{flap}_K(i, \delta) := (1+\delta)H_i \cap \bigcap_{j\neq i} H_i 
	\quad\text{and}\quad
	D_K(\delta) := \cbra{x\in\R^n : \abs{\#\cbra{i : x\in\mathrm{flap}(K, i,\delta)}} > 1 }.\]
	We also define  
	$\uflap_K(i,\delta) := \flap_K(i,\delta) \setminus D_K(\delta)$
	and the set
	\[R_K(i) := \{tv^{(i)} : t\geq \theta_i\} + (\partial H_i \cap K) \]
	where ``$+$'' here denotes the Minkowski sum.
	We will omit dependence on $K$ and write $\flap(i,\delta)$, $D(\delta)$, $\uflap(i,\delta)$ , and $R(i)$ for readability. It is easy to check that 
	\[
	\vol\pbra{D(\delta)} = O(\delta^2)
	\quad\text{and that}\quad
	\vol(R(i) \cap R(j)) = 0
	\]
	for $i\neq j$. Finally, we have 
	\[\frac{\vol\pbra{\uflap(i,\delta)}}{\vol\pbra{R(i)}} \geq \]
	
	\[\red{TODO: Influence calculation.}\]
\end{proofof}

\begin{proofof}{\Cref{prop:size-to-width}}
	\red{TODO}.
\end{proofof}

\begin{proposition} \label{prop:influence-width-ub}
	For $w>0$, let $K\sse\R^n$ be an intersection of (possibly infinitely many) halfspaces of the form 
	\[
	K = \bigcap_{i=1}^s H_i 
	\qquad\text{where}\qquad 
	H_i := \{x\in\R^n : \abra{x,v_i} \leq w\}
	\]
	for unit vectors $v_i \in \S^{n-1}$, and furthermore suppose $0^n\in K$.  Then we have 
	\[\TInf[K] \leq O(w^2).\]
\end{proposition}
